# Supplementary material for: Towards Practical Overlay Networks for Decentralized Federated Learning
Source: arXiv:2409.05331 source file (2024-09-09)
Supplement: Supplementary file 1 [file 7.appendix.tex]

\section*{Appendix}
\begin{figure*}
    \centering
    \begin{subfigure}[b]{0.30\textwidth}
        \centering
        \includegraphics[width=\textwidth]{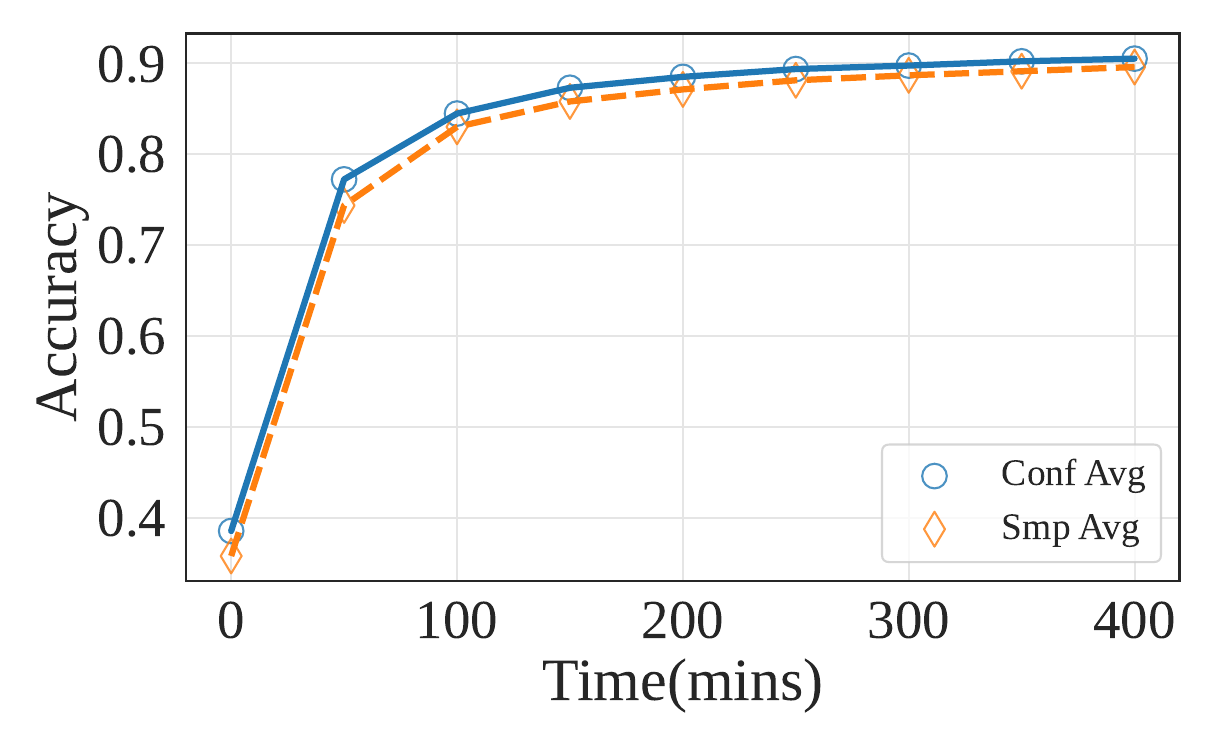}
        \caption{\footnotesize MNIST.$\alpha_d = 0.5,\alpha_c = 0.5$}
        \label{fig:confacc-m-n100d10s3}
    \end{subfigure}
    \begin{subfigure}[b]{0.30\textwidth}
        \centering
        \includegraphics[width=\textwidth]{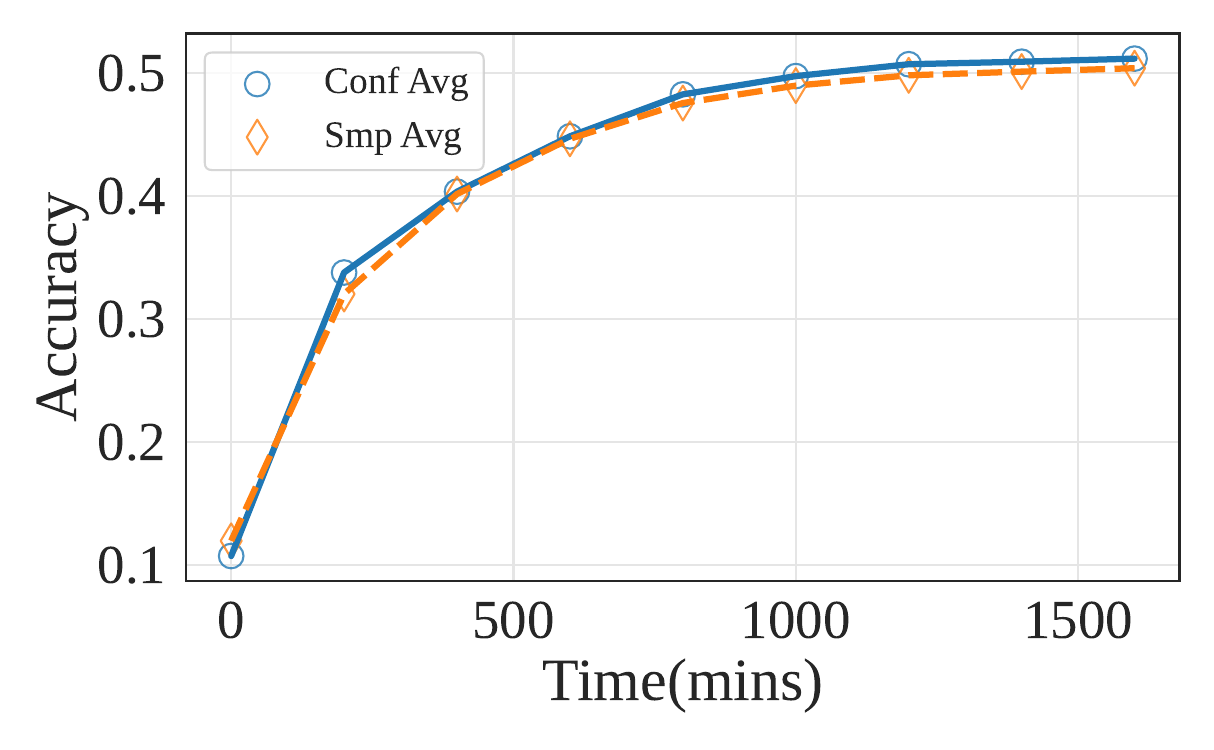}
        \caption{\footnotesize CIFAR-10.$\alpha_d = 1,\alpha_c = 0$}
        \label{fig:confacc-c-n100d10s8}
    \end{subfigure}
    \begin{subfigure}[b]{0.30\textwidth}
        \centering
        \includegraphics[width=\textwidth]{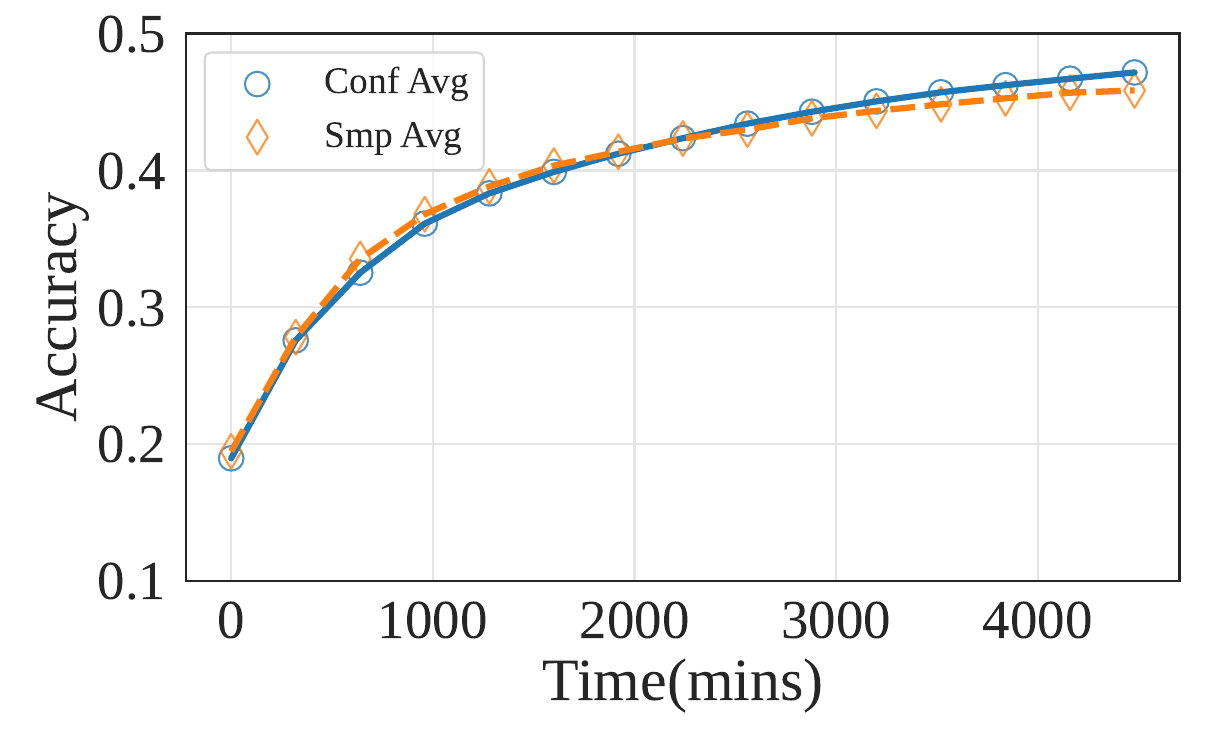}
        \caption{\footnotesize Shakespeare.$\alpha_d = 0,\alpha_c = 1$}
        \label{fig:confacc-s-n100d10}
    \end{subfigure}
    \begin{subfigure}[b]{0.30\textwidth}
        \centering
        \includegraphics[width=\textwidth]{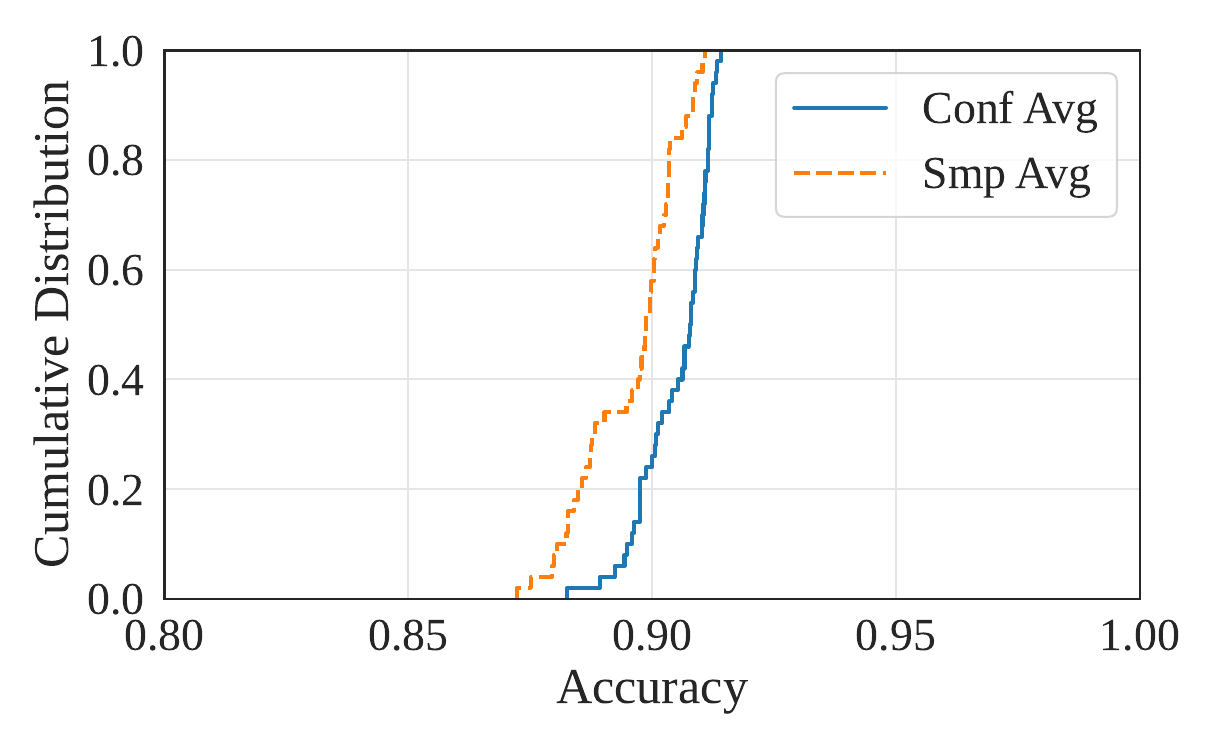}
        \caption{\footnotesize MNIST. Accuracy distribution}
        \label{fig:confacc-m-n100d10s3}
    \end{subfigure}
    \begin{subfigure}[b]{0.30\textwidth}
        \centering
        \includegraphics[width=\textwidth]{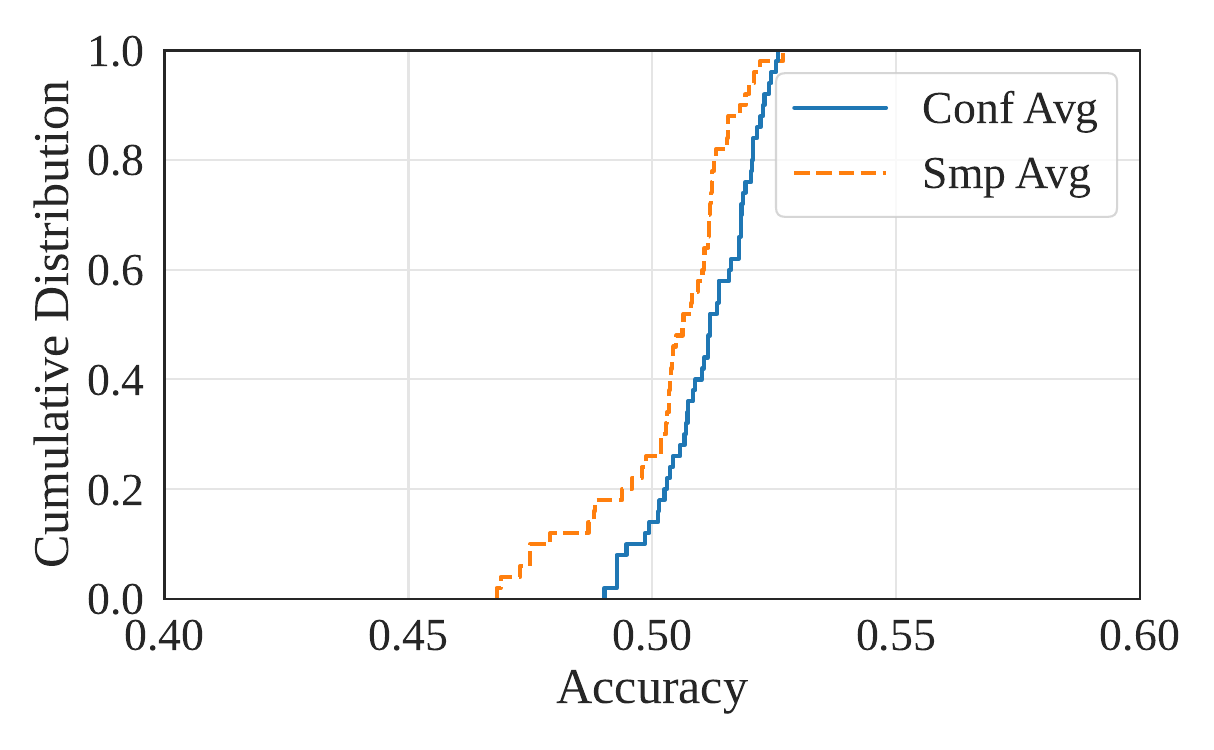}
        \caption{\footnotesize CIFAR-10. Accuracy distribution}
        \label{fig:confcdf-c-n100d10s8}
    \end{subfigure}
    \begin{subfigure}[b]{0.30\textwidth}
        \centering
        \includegraphics[width=\textwidth]{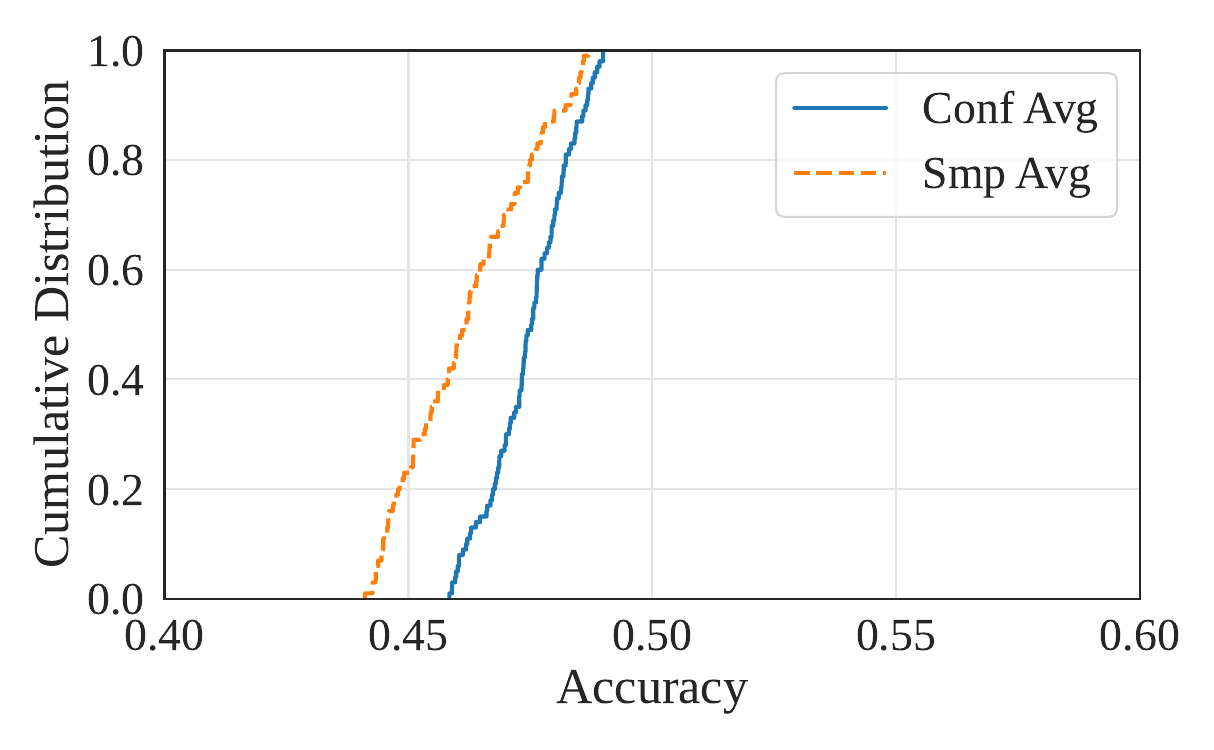}
        \caption{\footnotesize Shakespeare. Accuracy distribution}
        \label{fig:confcdf-s-n100d10}
    \end{subfigure}%\vspace{-1ex}
   \caption{Accuracy   with varying confidence settings for different datasets}
   \label{fig:confcdf}\vspace{-3ex}
\end{figure*}
The proof of Lemma 1:

\textbf{Lemma 1.}
\textit{In a ring space of a correct FedLay network and a given coordinate $x$, if a node $v$ is not the node that has the smallest circular distance to $x$ in the space, then $v$
must have an adjacent node $w$ on the ring such that $CD(x, x^v)>CD(x, x^{w})$, where $x^v$ is $v$'s coordinate.}

\begin{proof}
Let $p$ be the node with the smallest circular distance to  $x$ in the space. Consider the two arcs between $x$ and $x^v$. 
At least one of them has a length no longer than 0.5. Let that arc be $\wideparen{x^v, x}$ with length $L(\wideparen{x^v, x})$. $CD(x^v, x)=L(\wideparen{x^v, x})\leq 0.5$.

If $p$ is on $\wideparen{x^v, x}$, consider the arc between $v$ and $p$, $\wideparen{x^v, x^p}$, as a part of $\wideparen{x^v, x}$.  If $v$ has an adjacent node $q$ whose coordinate 
is on $\wideparen{x^v, x^p}$, then $L(\wideparen{x, x^q})<L(\wideparen{x^v, x})\leq 0.5$. Hence, $CD(x^v,x)>CD(x^q,x)$. The lemma holds in this situation.
If $v$ has no adjacent node on $\wideparen{x^v, x^p}$, then there must be no node on the arc $\wideparen{x^v, x^p}$. Hence, $v$ and $p$ are adjacent nodes. 
Since $p$ is the node closest to $x$,  $v$ does have an adjacent node $p$ that is closer to $x$. The lemma also holds in this situation.

If $p$ is not on $\wideparen{x^v, x}$, consider the arc $\wideparen{x^v, x, x^p}$. The arc $\wideparen{x, x^p}$ is a part of $\wideparen{x^v, x, x^p}$, and we have $L(\wideparen{x, x^p})<L(\wideparen{x^v, x})$, because $p$ is the closest node to $x$. If $v$ has an adjacent node $q$ whose coordinate 
is on $\wideparen{x^v, x, x^p}$, then $L(\wideparen{x, x^q})<L(\wideparen{x^v, x})\leq 0.5$. Hence, $CD(x^v,x)>CD(x^q,x)$. The lemma holds in this situation.
If $v$ has no adjacent node on $\wideparen{x^v, x, x^p}$, then $v$ and $p$ are adjacent nodes. Since $p$ is the node closest to $x$,  $v$ does have an adjacent node $p$ that is closer to $x$. The lemma also holds in this situation.

Therefore in all cases, the lemma holds.
\end{proof}

The proof of Theorem 2:

\textbf{Theorem 2.}
\textit{Consider a correct FedLay network and a node $u$ fails. 
When a node $p$ detects the failure of its adjacent node $u$ in Space $i$, it sends \textit{Neighbor\_repair} to the destination coordinate $x_i^u$ in the opposite direction of $u$. 
When \textit{Neighbor\_repair} stops at a node $q$, $q$ is another adjacent node of $u$ in Space $i$ before $u$'s failure. 
}
\begin{proof}
We first discuss the case that \textit{Neighbor\_repair} is sent in the counterclockwise direction. The case of clockwise direction can be proved in the same way. 

Let $q$ be another adjacent node of $u$ in Space $i$ before $u$'s failure. 

Let $v$ be the current node that receives \textit{Neighbor\_repair}. 
%Consider the length of the arc from $x_i^v$ to $x_i^u$ in the counterclockwise direction $L(\wideparen{x_i^v, x_i^u})$.  
If $v \neq q$, $v$ has at least one neighbor $w$, such that $L(\wideparen{x_i^w, x_i^u})<L(\wideparen{x_i^v, x_i^u})$. 
Hence, \textit{Neighbor\_repair} will not stop if $v \neq q$.
$v$ will forward \textit{Neighbor\_repair} to the neighbor $w'$ and $L(\wideparen{x_i^{w'}, x_i^u})\leq L(\wideparen{x_i^w, x_i^u}) < L(\wideparen{x_i^v, x_i^u})$.

Therefore after each hop, the arc length $L(\wideparen{x_i^v, x_i^u})$ strictly decreases.
Hence, \textit{Neighbor\_repair} will not experience a loop. 
Since there are a limited number of nodes, \textit{Neighbor\_repair} will stop at $q$. 
\end{proof}

Fig.~\ref{fig:confcdf} show the accuracy with varying confidence settings for different datasets. 
\begin{figure*}
    \centering
    \begin{subfigure}[b]{0.30\textwidth}
        \centering
        \includegraphics[width=\textwidth]{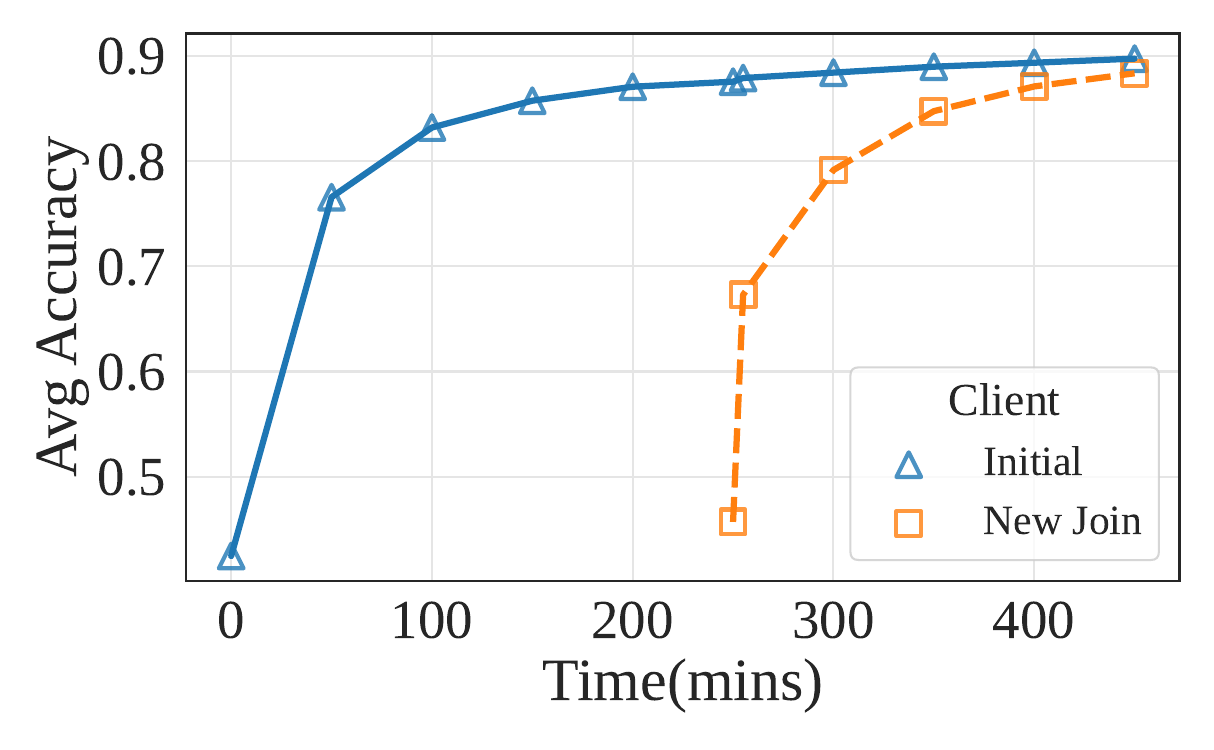}%\vspace{-2ex}
        \caption{\footnotesize  Accuracy under churn for MNIST.}
        \label{fig:join-m-n5050d10s4}
    \end{subfigure}
    \begin{subfigure}[b]{0.30\textwidth}
        \centering
        \includegraphics[width=\textwidth]{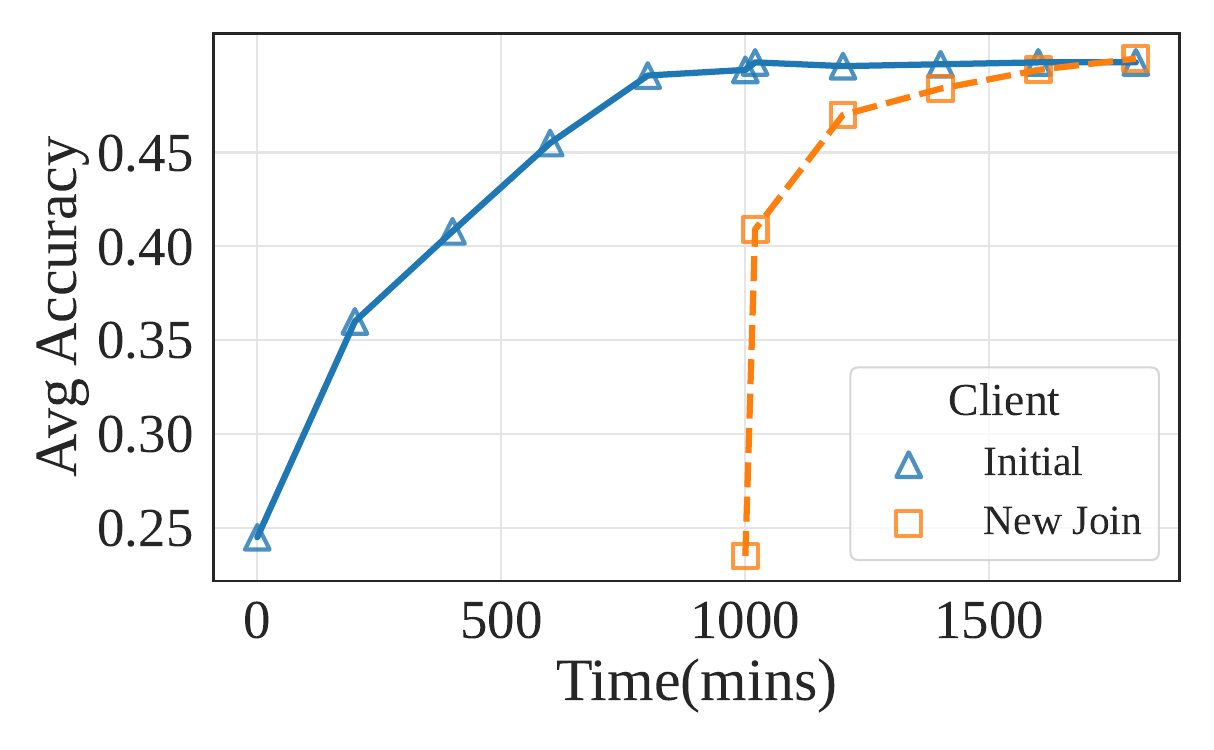}%\vspace{-2ex}
        \caption{\footnotesize  Accuracy under churn for CIFAR-10.}
        \label{fig:join-c-n5050d10s8}
    \end{subfigure}
    \begin{subfigure}[b]{0.30\textwidth}
        \centering
        \includegraphics[width=\textwidth]{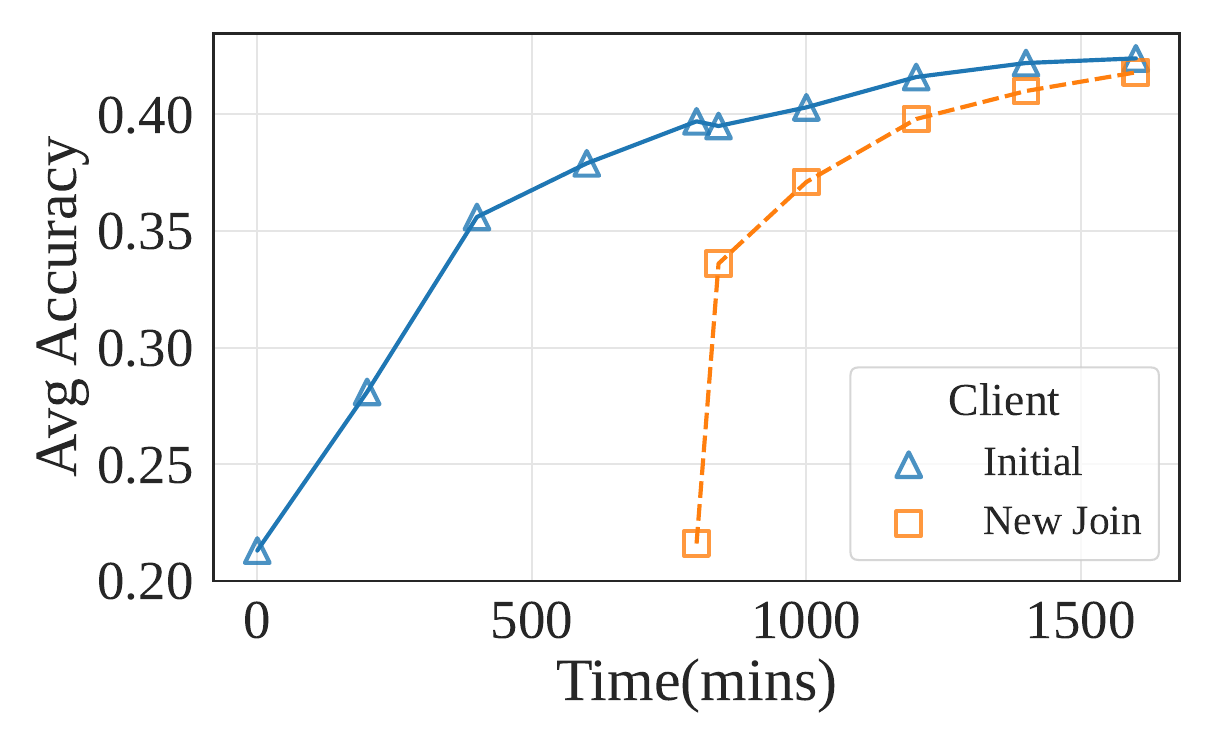}%\vspace{-2ex}
        \caption{\footnotesize Accuracy under churn for Shakespeare.}
        \label{fig:join-s-n5050}
    \end{subfigure} 
    \begin{subfigure}[b]{0.30\textwidth}
        \centering
        \includegraphics[width=\textwidth]{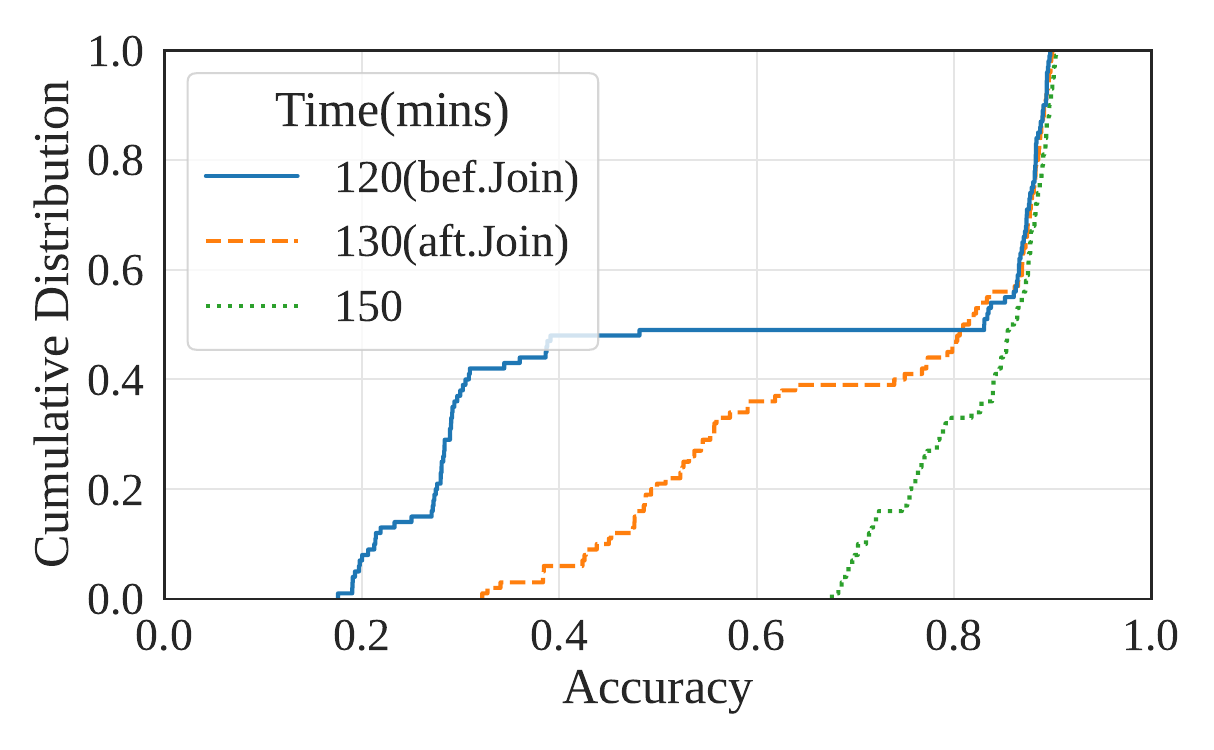}%\vspace{-2ex}
        \caption{\footnotesize Accuracy distribution for MNIST}
        \label{fig:joincdf-m-n5050d10s4}
    \end{subfigure}
    \begin{subfigure}[b]{0.30\textwidth}
        \centering
        \includegraphics[width=\textwidth]{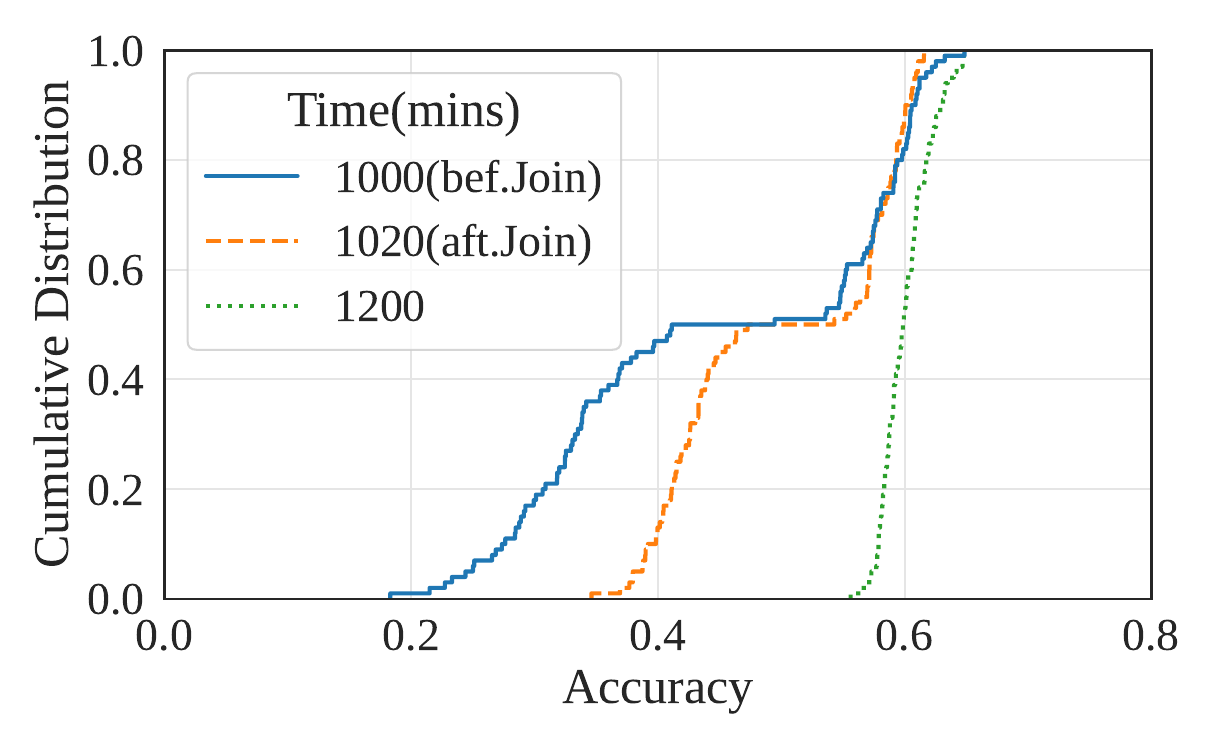}%\vspace{-2ex}
        \caption{\footnotesize Accuracy distribution for CIFAR-10}
        \label{fig:joincdf-c-n5050d10s8}
    \end{subfigure}
    \begin{subfigure}[b]{0.30\textwidth}
        \centering
        \includegraphics[width=\textwidth]{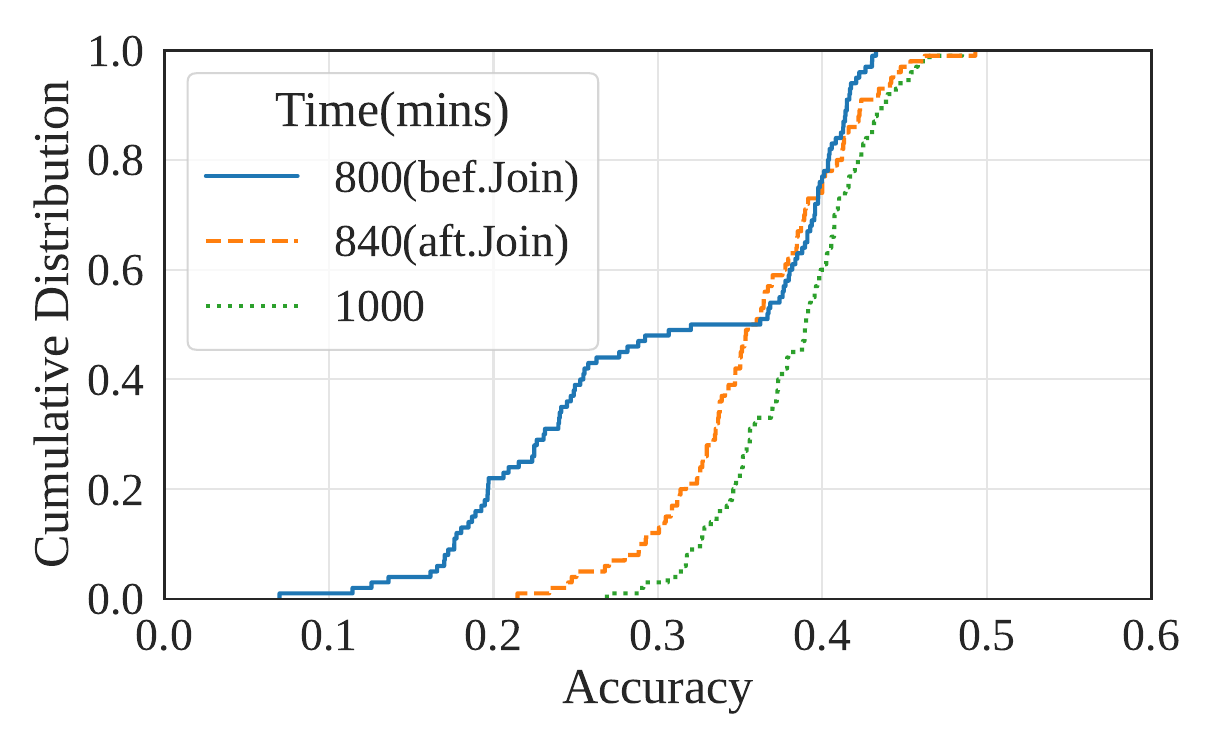}%\vspace{-2ex}
        \caption{\footnotesize Accuracy distribution for Shakespeare}
        \label{fig:joincdf-s-n5050d10}
    \end{subfigure}%\vspace{-1ex}
     \caption{Accuracy of FedLay under churn (50 new clients join a 50-client FedLay). For MNIST, CIFAR-10, and Shakespeare,  clients join at 250, 1000 and 800 mins respectively.}
   \label{fig:join-acc}%\vspace{-4ex}
\end{figure*}

Figure \label{fig:join-acc} shows the accuracy of FedLay under an extreme case of churn (50 new clients join a 50-client FedLay) for  MNIST, CIFAR-10, and Shakespeare.
